# Supplementary material for: Beyond the Known: Decision Making with Counterfactual Reasoning Decision Transformer
Source: arXiv:2505.09114 source file (2025-05-14)
Supplement: Supplementary file 2 [file varying_action_selection.tex]

In this section, we provide an explanation of the variations of the action selection method and how they were implemented. We have 4 variations: without comparing the returns-to-go $g$ (W/o comparing $g$), without using the uncertainty filter (W/o $U^\alpha(\textbf{S}_k)$), simply sampling the mean action $a$, and sampling the mean action with a small   

% DT & 62.1±2.2 \\
%       W/o comparing $g$ & 67.4±2.1 \\
%       W/o $U^\alpha(\textbf{S}_k)$ & 69.6±2.8 \\
%       $a$ & 68.4±3.45 \\
%       $a + \text{noise}~\epsilon$ & 69.3±4.4 \\
